# Supplementary material for: Atomic Confinement Potentials and the Generation of Numerical Atomic Orbitals
Source: arXiv:2505.09540 ancillary file (2025-07-30)
Supplement: Supplementary file 1 [file SI.pdf]

# Supporting Information for "Atomic Confinement Potentials"

Hugo Åström and Susi Lehtola[a)]

*University of Helsinki, Department of Chemistry, Faculty of Science, P.O. Box 55 (A.I. Virtanens plats 1), FI-00014 University of Helsinki, Finland*

[a)] Electronic mail: susi.lehtola@alumni.helsinki.fi

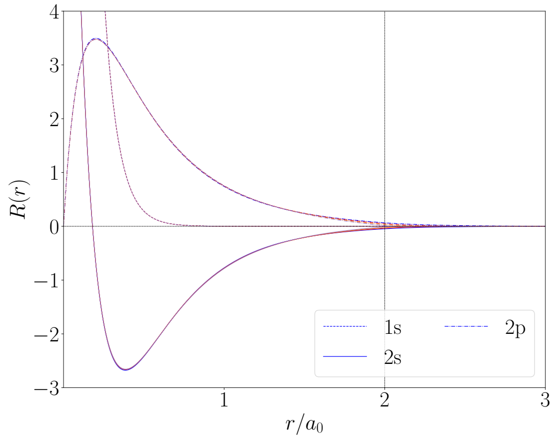


Figure 1: The radial part of the 1s, 2s and 2p orbitals of Mg in the finite-barrier potential for $r_0 = 2a_0$.

# I. FINITE-BARRIER POTENTIAL

## A. Contracting the orbitals

### *1. Core orbitals*

The radial parts of the core orbitals of Mg in the finite-barrier potential are plotted in fig. 1 and of Ca in fig. 2.

### *2. Valence orbitals*

The radial part of the 4s orbital of Ca in the finite-barrier potential is plotted in fig. 3.

## B. Truncating the grid

The radial density of the 3s orbital of Mg in the finite-barrier potential with $r_\infty = 15a_0$, as well as with a truncated radial grid is plotted in fig. 4 for $r_0 = 2a_0$ and in fig. 5 for $r_0 = 3a_0$, now in semilogarithmic scale.

The values of $r_\infty$ that result in a 1 μ$E_h$ energy increase from the converged radial grid with $r_\infty = 15a_0$ for Ca in the finite-barrier potential are shown in table I.

The radial density of the 4s orbital of Ca in the finite-barrier potential with $r_\infty = 15a_0$

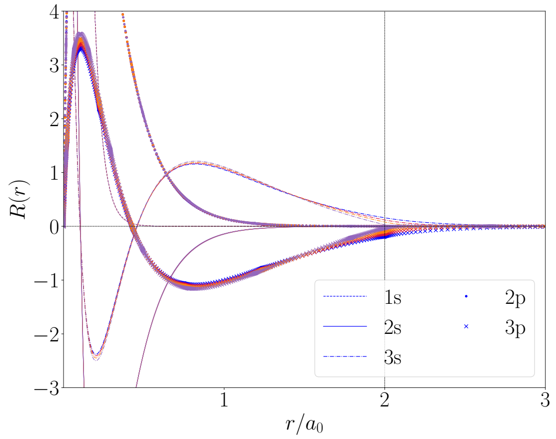


(a)

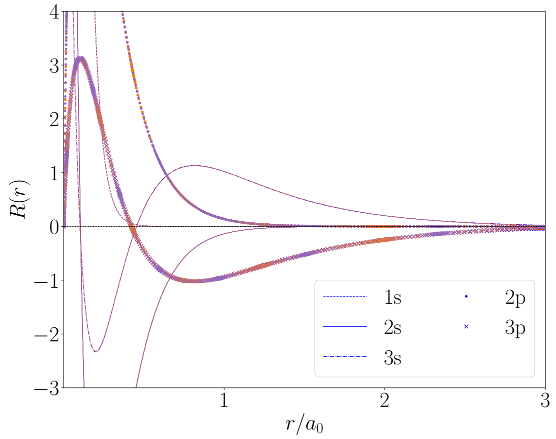


(b)

Figure 2: The radial part of the 1s, 2s, 3s, 2p, and 3p orbitals of Ca in the finite-barrier potential for $r_0 = 2a_0$ (fig. 2a) and $r_0 = 3a_0$ (fig. 2b).

and $r_0 \in \{2.0, 3.0, 4.0\}a_0$ is plotted in fig. 6. Analogous plots with a truncated radial grid are found in fig. 7.

### C. Approaching the hard-wall limit

The 4s orbital of Ca in the finite-barrier potential with $r_0 = 5a_0$ and increasing barrier heights as well as the hard-wall potential with $r_\infty = 5a_0$ is depicted in fig. 8.

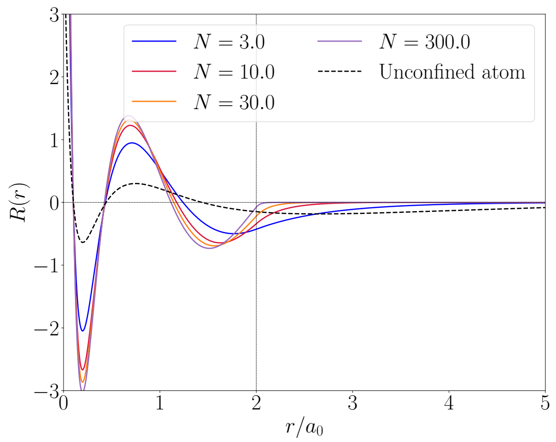


(a)

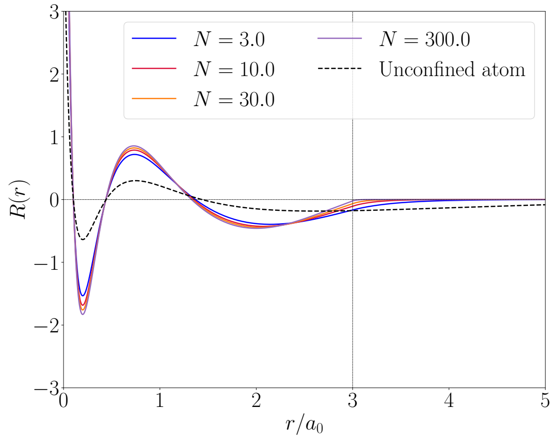


(b)

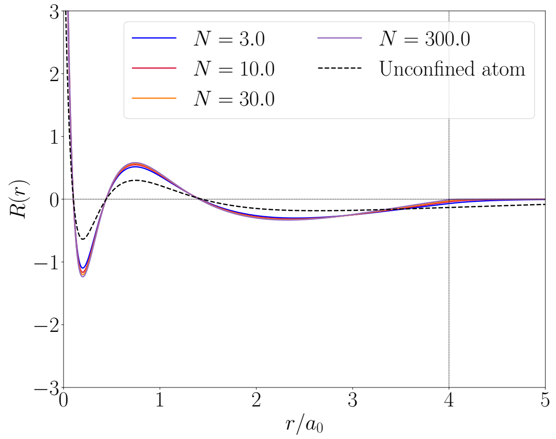


(c)

Figure 3: The radial part of the 4s orbital of Ca in the finite-barrier potential for $r_0 = 2a_0$ (fig. 3a), $r_0 = 3a_0$ (fig. 3b), and $r_0 = 4a_0$ (fig. 3c).

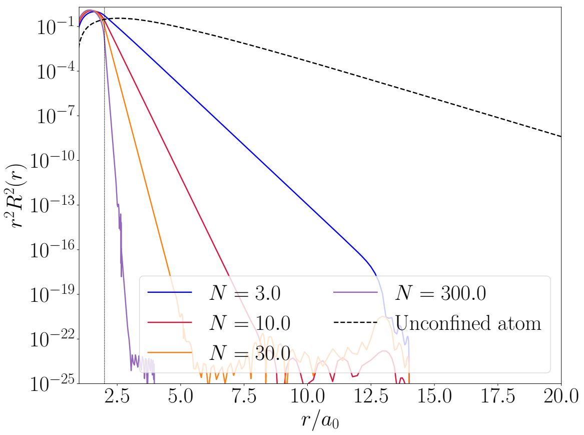


(a)

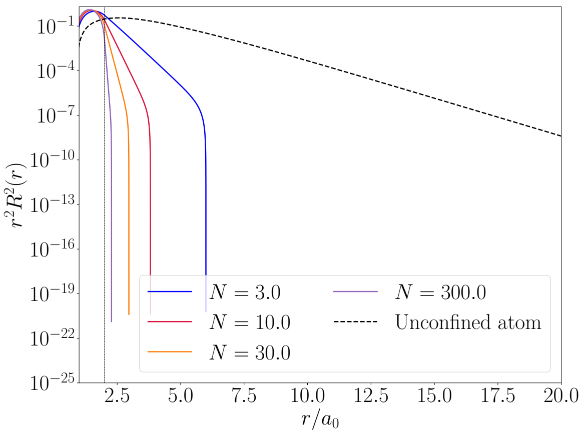


(b)

Figure 4: The radial density of the 3s orbital of Mg in the finite-barrier potential for $r_0 = 2a_0$ with $r_\infty = 15a_0$ (fig. 4a) and a truncated radial grid (fig. 4b).

## II. POLYNOMIAL AND EXPONENTIAL POTENTIALS

### A. Contracting the orbitals

#### *1. Core orbitals*

The radial parts of the core orbitals of Mg in the polynomial potential are plotted in fig. 9 and of Ca in fig. 10. Analogous plots for the exponential potential are depicted in fig. 11 and fig. 12 for the Mg and Ca atoms respectively.

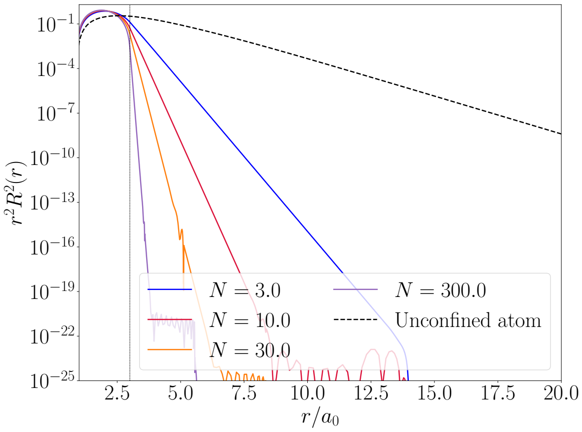


(a)

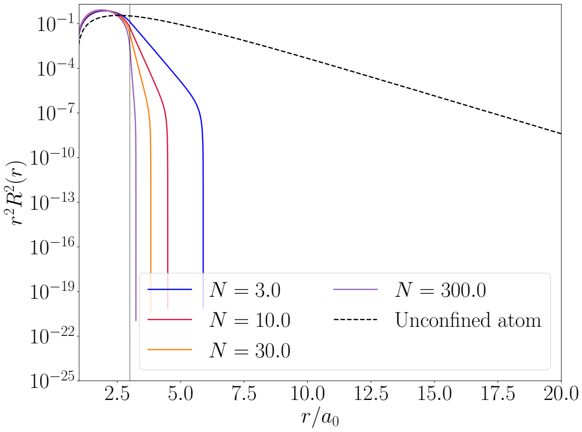


(b)

Figure 5: The radial density of the 3s orbital of Mg in the finite-barrier potential for $r_0 = 3a_0$ with $r_\infty = 15a_0$ (fig. 5a) and a truncated radial grid (fig. 5b).

### *2. Valence orbitals*

The radial part of the 4s orbital of Ca are found in figs. 13 and 14 for the polynomial and exponential potentials respectively.

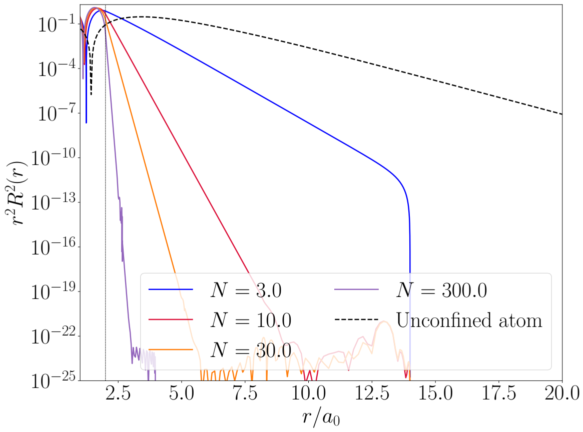


(a)

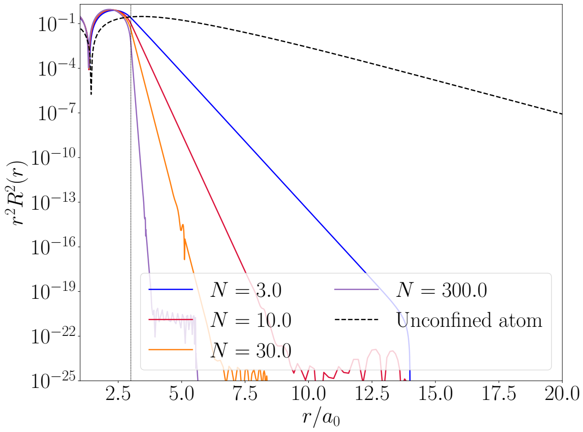


(b)

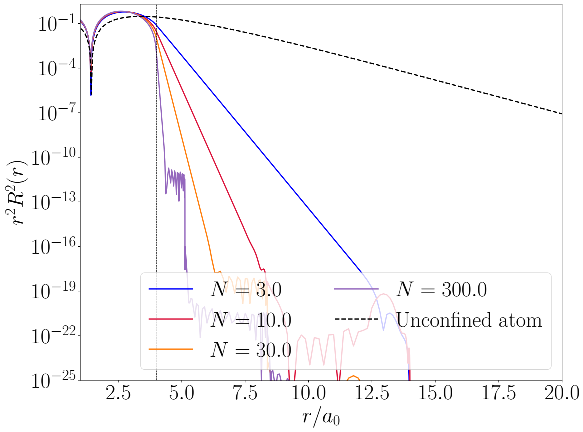


(c)

Figure 6: The radial density of the 4s orbital of Ca in the finite-barrier potential with $r_\infty = 15a_0$ and $r_0 = 2a_0$ (fig. 6a), $r_0 = 3a_0$ (fig. 6b), and $r_0 = 4a_0$ (fig. 6c).

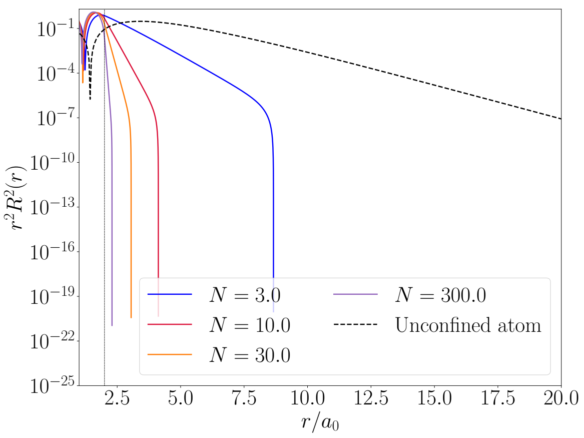


(a)

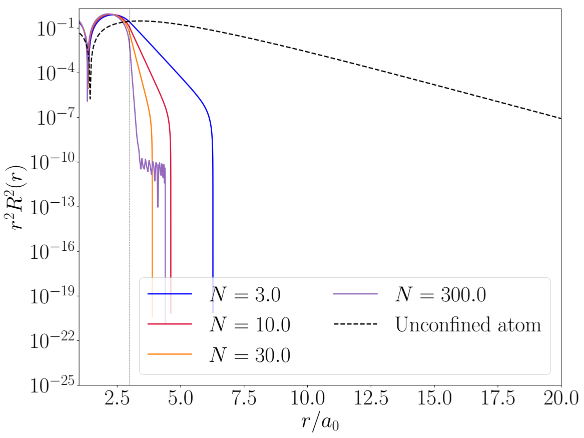


(b)

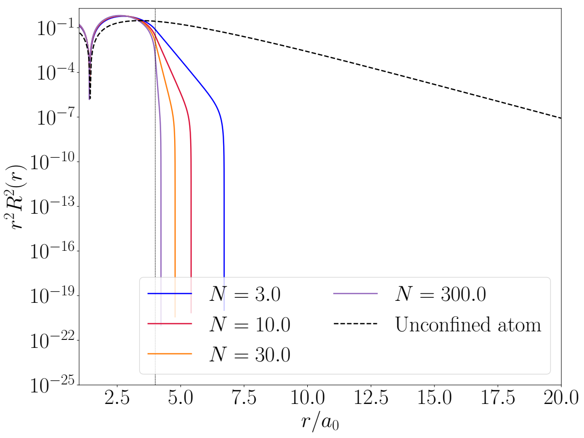


(c)

Figure 7: The radial density of the 4s orbital of Ca in the finite-barrier potential with a truncated radial grid and $r_0 = 2a_0$ (fig. 7a), $r_0 = 3a_0$ (fig. 7b), and $r_0 = 4a_0$ (fig. 7c).

| | LIP | | | HIP | | | HIP' | | |
|---|---|---|---|---|---|---|---|---|---|
| $V_0$ | 2.0 | 3.0 | 4.0 | 2.0 | 3.0 | 4.0 | 2.0 | 3.0 | 4.0 |
| 3 | 8.66 | 6.27 | 6.71 | 8.66 | 6.27 | 6.71 | 8.67 | 6.28 | 6.73 |
| 10 | 4.12 | 4.61 | 5.41 | 4.12 | 4.61 | 5.41 | 4.13 | 4.62 | 5.42 |
| 30 | 3.05 | 3.88 | 4.78 | 3.05 | 3.88 | 4.78 | 3.05 | 3.89 | 4.79 |
| 300 | 2.30 | 4.39 | 4.23 | 2.30 | 3.26 | 4.23 | 2.30 | 3.26 | 4.23 |

Table I: Values of practical infinity ($r_\infty$) in $a_0$ resulting in a 1 µE$_\mathrm{h}$ energy increase from a converged radial grid for the Ca atom in finite-barrier confinement with $r_0 \in \{2.0, 3.0, 4.0\}a_0$. LIP: Lagrange interpolating polynomial, HIP: Hermite interpolating polynomial, HIP': HIP with zero derivative at $r_\infty$.

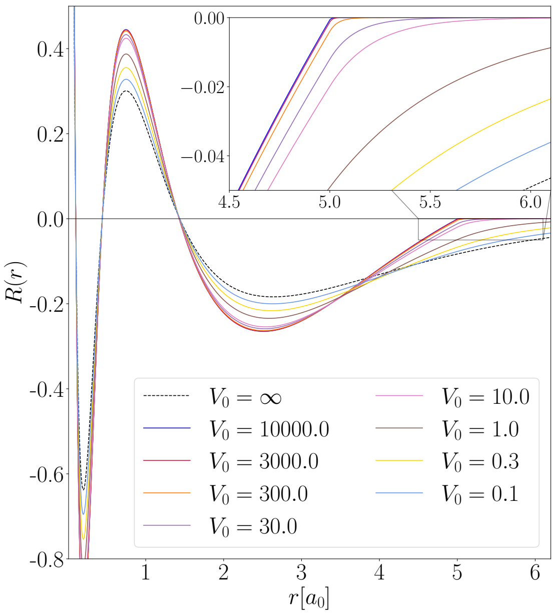


Figure 8: The 4s orbital of Ca in the finite-barrier potential with various $V_0$ and $r_0 = 5a_0$, as well as the hard-wall potential with $r_\infty = 5a_0$.

## B. Truncating the grid

The radial density of the 3s orbital of Mg in the polynomial potential with $r_\infty = 15a_0$, as well as with a truncated radial grid is plotted in fig. 15 for $r_0 = 2a_0$ and in fig. 16 for

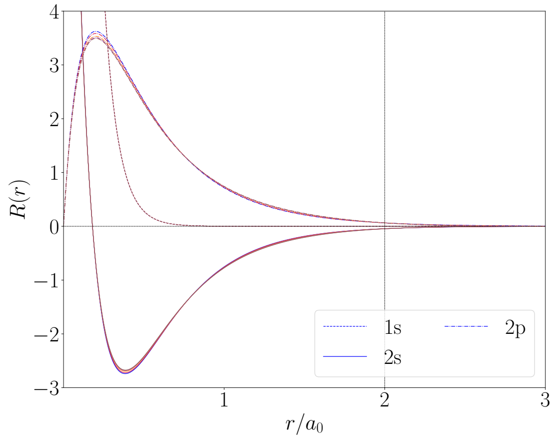


Figure 9: The radial part of the 1s, 2s and 2p orbitals of Mg in the polynomial potential for $r_0 = 2a_0$.

$r_0 = 3a_0$, now in semilogarithmic scale. Analogous plots for the exponential potential are found in fig. 17 and fig. 17 respectively.

The values of $r_\infty$ that result in a 1 µ$E_h$ energy increase from the converged radial grid with $r_\infty = 15a_0$ for Ca in the polynomial potential are shown in table II and for the exponential potential in table III.

The radial density of the 4s orbital of Ca in the polynomial potential with $r_\infty = 15a_0$ and $r_0 \in \{2.0, 3.0, 4.0\}a_0$ is plotted in fig. 19 and with a truncated radial grid in fig. 20. Analogous plots for the exponential potential are found in fig. 21 and fig. 22 respectively.

### C. Approaching the hard-wall limit

Values of $r_\infty$ in $a_0$ that minimize the norm between the 4s orbital of the Ca atom in the shifted polynomial and exponential potentials and the hard-wall potential, for various values of $N$, $r_0$ and $\delta$, are shown in table IV.

The 3s orbital of Mg in the shifted potentials for various values of $r_0$ and $\delta$ together with the hard-wall confined orbital is shown in figs. 23 to 25 for $N \in \{2, 4, 6\}$. Analogous plots for the 4s orbital of Ca are shown in figs. 26 to 29 for $N \in \{2, 4, 6, 10\}$.

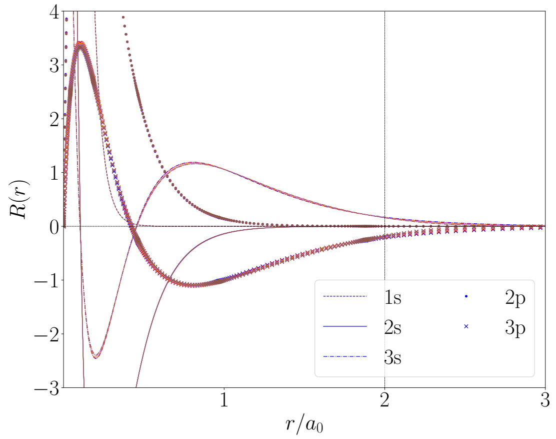


(a)

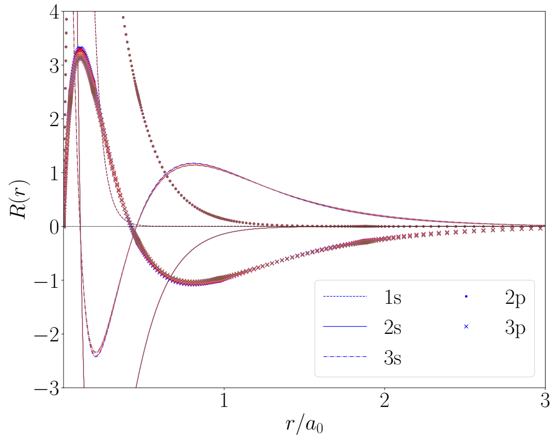


(b)

Figure 10: The radial part of the 1s, 2s, 3s, 2p, and 3p orbitals of Ca in the polynomial potential for $r_0 = 2a_0$ (fig. 10a) and $r_0 = 3a_0$ (fig. 10b).

## III. SINGULAR POTENTIALS

### A. Orbital contraction

The 4s orbital of Ca confined by the singular potentials with $n \in \{1, 2, 3\}$ with the FHI-AIMS "light" and "tight" default values of $r_i$ and $r_c$ and various $V_0$ is shown in fig. 30.

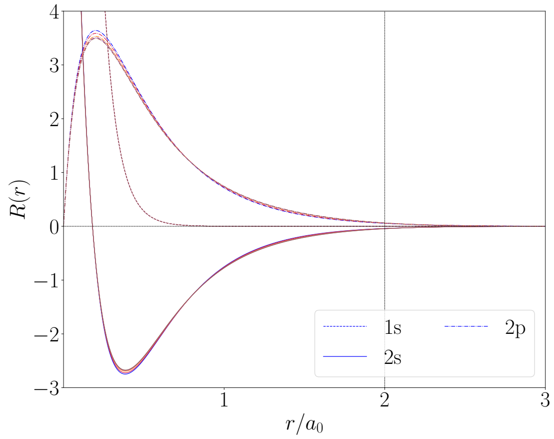


Figure 11: The radial part of the 1s, 2s and 2p orbitals of Mg in the exponential potential for $r_0 = 2a_0$.

| | LIP | | | HIP | | | HIP' | | |
|---|---|---|---|---|---|---|---|---|---|
| $N$ | 2.0 | 3.0 | 4.0 | 2.0 | 3.0 | 4.0 | 2.0 | 3.0 | 4.0 |
| 1 | 7.66 | 8.42 | 8.99 | 7.66 | 8.42 | 8.99 | 7.68 | 8.44 | 9.01 |
| 2 | 5.80 | 6.82 | 7.63 | 5.80 | 6.82 | 7.63 | 5.81 | 6.83 | 7.65 |
| 4 | 4.41 | 5.60 | 6.62 | 4.41 | 5.60 | 6.62 | 4.42 | 5.61 | 6.63 |
| 6 | 3.81 | 5.04 | 6.14 | 3.81 | 5.04 | 6.14 | 3.82 | 5.05 | 6.15 |
| 8 | 3.47 | 4.71 | 5.84 | 3.47 | 4.71 | 5.84 | 3.48 | 4.72 | 5.85 |
| 10 | 3.25 | 4.47 | 5.62 | 3.25 | 4.48 | 5.62 | 3.25 | 4.49 | 5.63 |

Table II: Values of practical infinity ($r_\infty$) in $a_0$ resulting in a 1 μE$_\mathrm{h}$ energy increase from a converged radial grid for the Ca atom in polynomial confinement with $r_0 \in \{2.0, 3.0, 4.0\}a_0$. LIP: Lagrange interpolating polynomial, HIP: Hermite interpolating polynomial, HIP': HIP with zero derivative at $r_\infty$.

### *1. Approaching the hard-wall limit*

The 4s orbital of Ca in the singular potential for $n \in \{1, 2, 3\}$ and various values of $r_c - r_i$ approaching the hard-wall limit is shown in fig. 31.

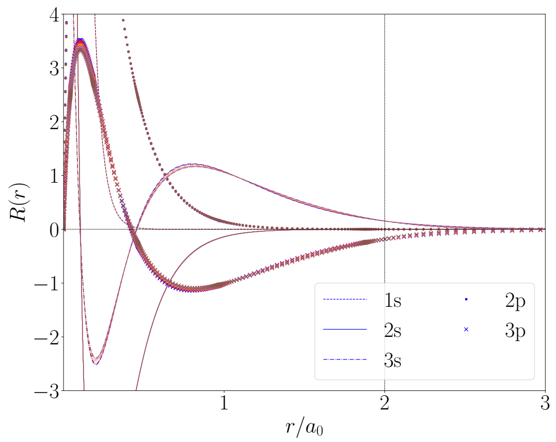


(a)

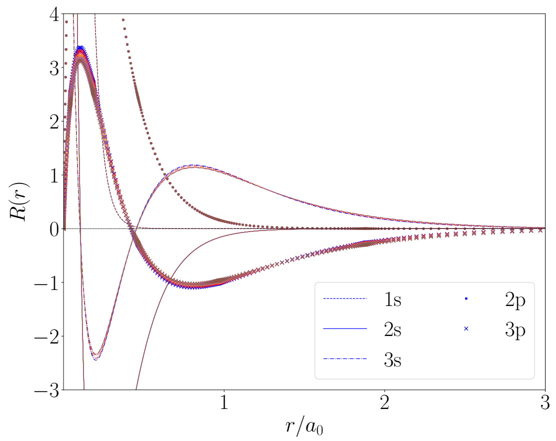


(b)

Figure 12: The radial part of the 1s, 2s, 3s, 2p, and 3p orbitals of Ca in the exponential potential for $r_0 = 2a_0$ (fig. 12a) and $r_0 = 3a_0$ (fig. 12b).

## B. Basis set truncation errors

The basis set truncation errors caused by confinement for the H–Xe atoms in the singular potential with $n = 2$ and the "light", "intermediate", and "tight" defaults in FHI-AIMS are shown in fig. 32.

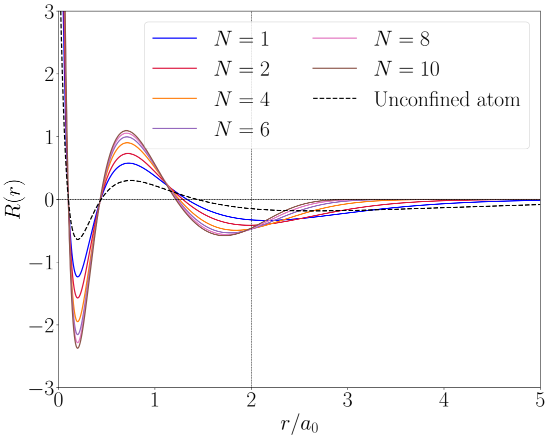


(a)

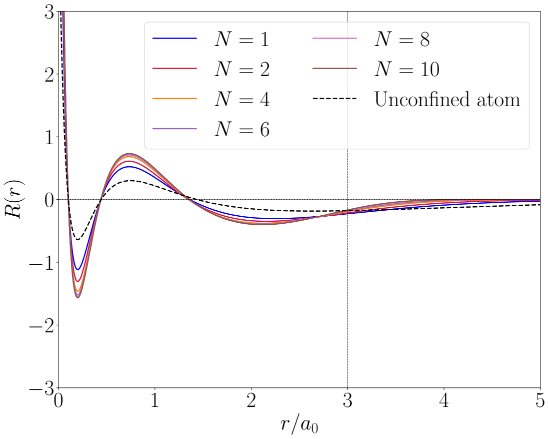


(b)

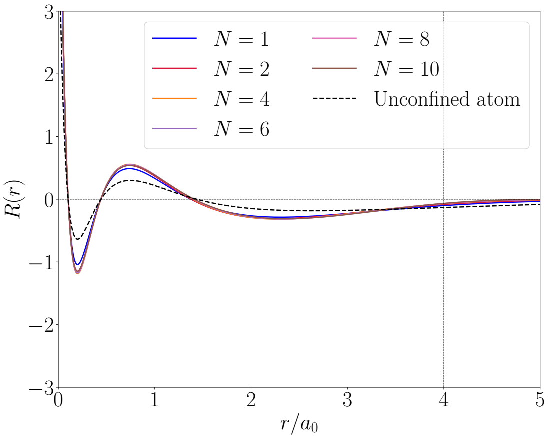


(c)

Figure 13: The radial part of the 4s orbital of Ca in the polynomial potential for $r_0 = 2a_0$ (fig. 13a), $r_0 = 3a_0$ (fig. 13b), and $r_0 = 4a_0$ (fig. 13c).

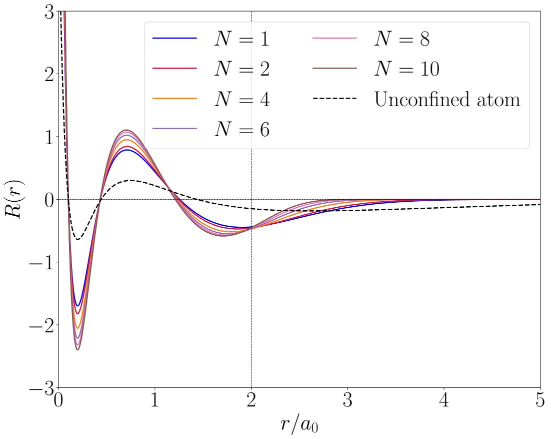


(a)

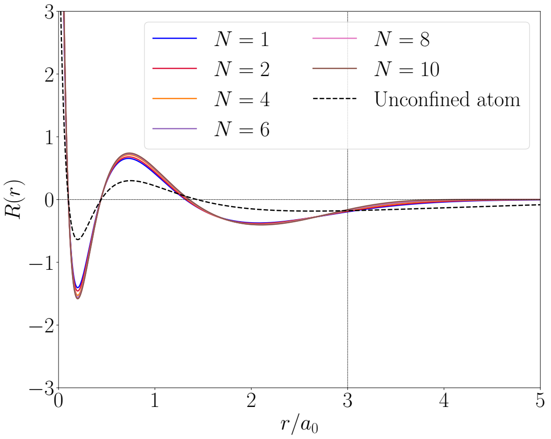


(b)

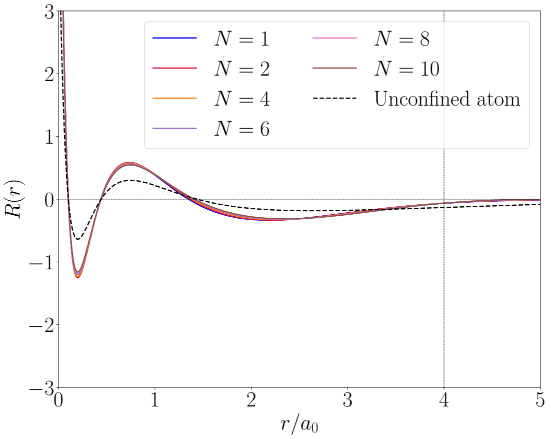


(c)

Figure 14: The radial part of the 4s orbital of Ca in the exponential potential for $r_0 = 2a_0$ (fig. 14a), $r_0 = 3a_0$ (fig. 14b), and $r_0 = 4a_0$ (fig. 14c).

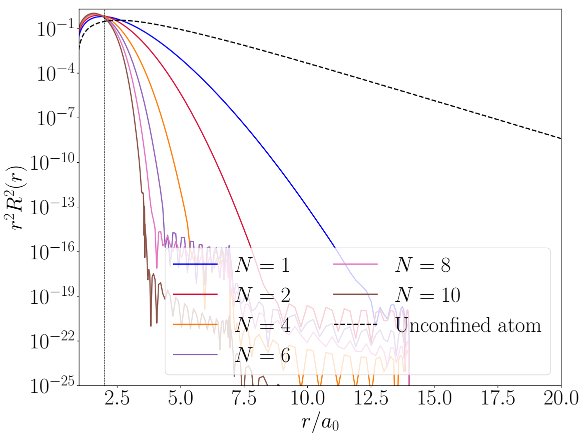


(a)

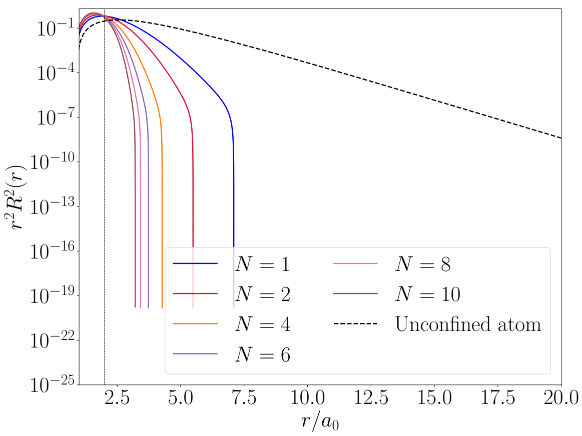


(b)

Figure 15: The radial density of the 3s orbital of Mg in the polynomial potential for $r_0 = 2a_0$ with $r_\infty = 15a_0$ (fig. 15a) and a truncated radial grid (fig. 15b).

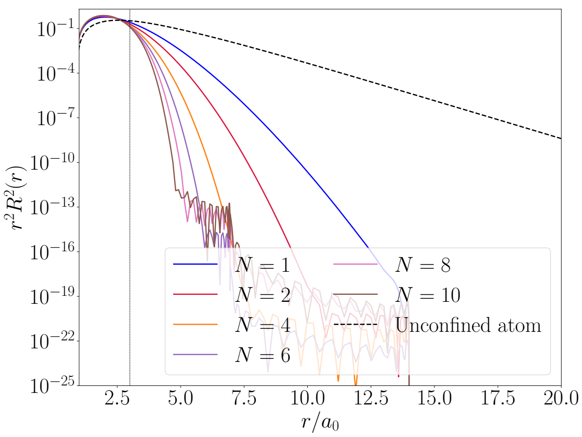


(a)

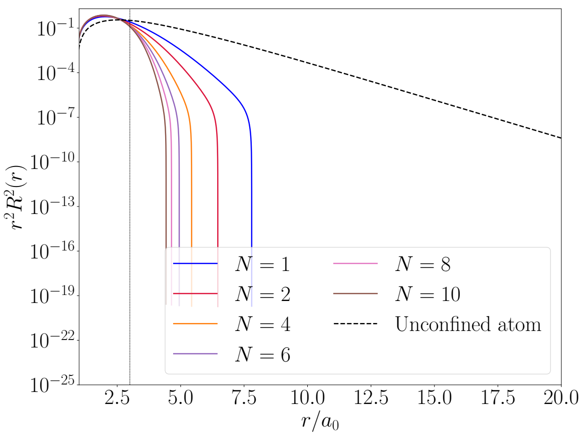


(b)

Figure 16: The radial density of the 3s orbital of Mg in the polynomial potential for $r_0 = 3a_0$ with $r_\infty = 15a_0$ (fig. 16a) and a truncated radial grid (fig. 16b).

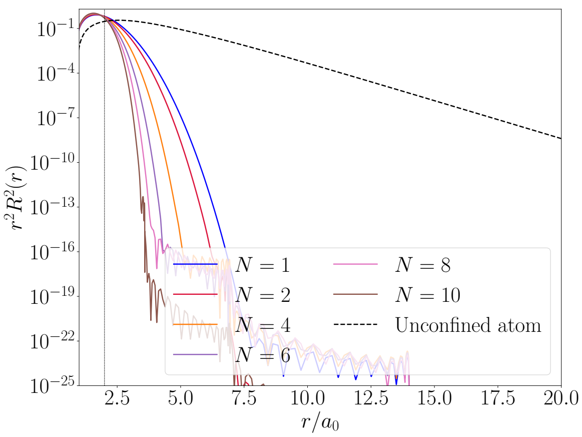


(a)

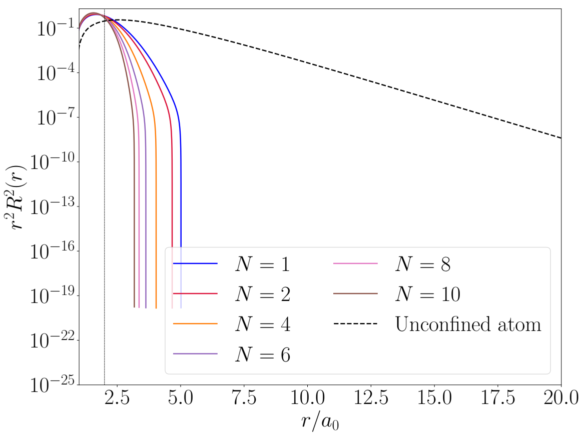


(b)

Figure 17: The radial density of the 3s orbital of Mg in the exponential potential for $r_0 = 2a_0$ with $r_\infty = 15a_0$ (fig. 17a) and a truncated radial grid (fig. 17b).

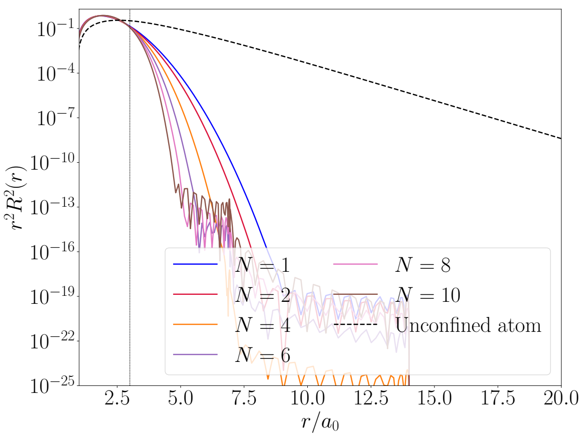


(a)

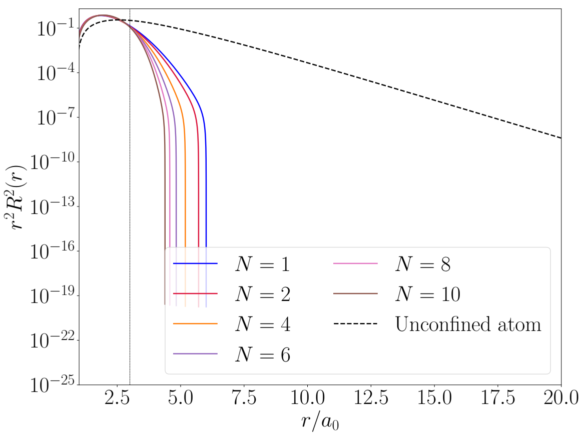


(b)

Figure 18: The radial density of the 3s orbital of Mg in the exponential potential for $r_0 = 3a_0$ with $r_\infty = 15a_0$ (fig. 18a) and a truncated radial grid (fig. 18b).

| | LIP | | | HIP | | | HIP’ | | |
|---|---|---|---|---|---|---|---|---|---|
| $N$ | 2.0 | 3.0 | 4.0 | 2.0 | 3.0 | 4.0 | 2.0 | 3.0 | 4.0 |
| 1 | 5.26 | 6.32 | 7.13 | 5.26 | 6.32 | 7.12 | 5.27 | 6.34 | 7.14 |
| 2 | 4.87 | 5.96 | 6.83 | 4.87 | 5.96 | 6.83 | 4.88 | 5.97 | 6.85 |
| 4 | 4.15 | 5.33 | 6.34 | 4.15 | 5.33 | 6.34 | 4.16 | 5.34 | 6.36 |
| 6 | 3.70 | 4.92 | 6.00 | 3.70 | 4.92 | 6.00 | 3.71 | 4.93 | 6.02 |
| 8 | 3.41 | 4.64 | 5.76 | 3.41 | 4.64 | 5.76 | 3.42 | 4.65 | 5.77 |
| 10 | 3.21 | 4.43 | 5.57 | 3.21 | 4.43 | 5.57 | 3.22 | 4.44 | 5.58 |

Table III: Values of practical infinity ($r_\infty$) in $a_0$ resulting in a 1 μ$E_h$ energy increase from a converged radial grid for the Ca atom in exponential confinement with $r_0 \in \{2.0, 3.0, 4.0\}a_0$. LIP: Lagrange interpolating polynomial, HIP: Hermite interpolating polynomial, HIP’: HIP with zero derivative at $r_\infty$.

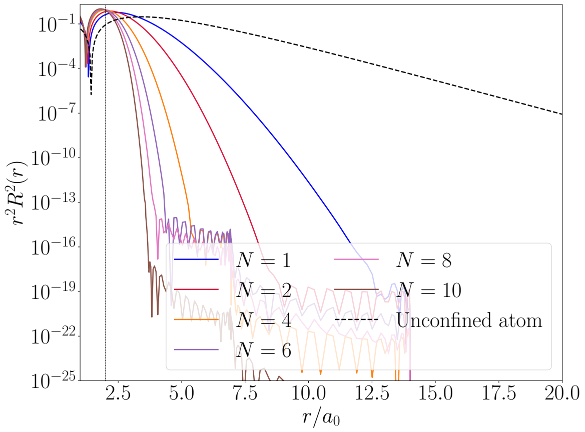


(a)

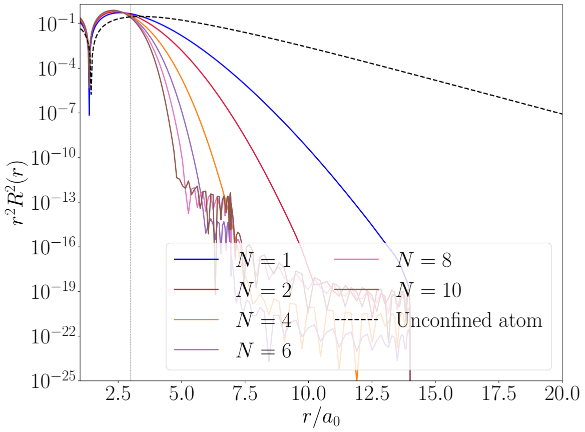


(b)

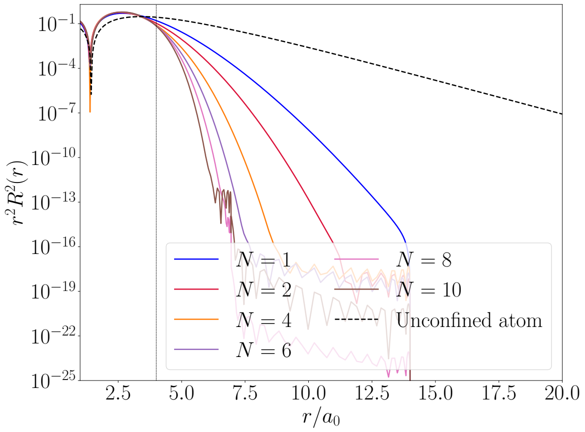


(c)

Figure 19: The radial density of the 4s orbital of Ca in the polynomial potential with $r_\infty = 15a_0$ and $r_0 = 2a_0$ (fig. 19a), $r_0 = 3a_0$ (fig. 19b), and $r_0 = 4a_0$ (fig. 19c).

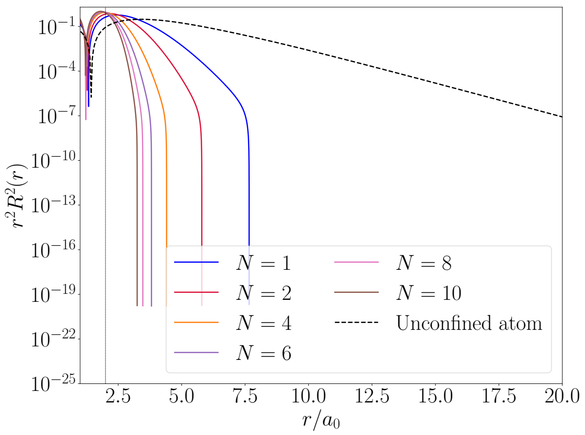


(a)

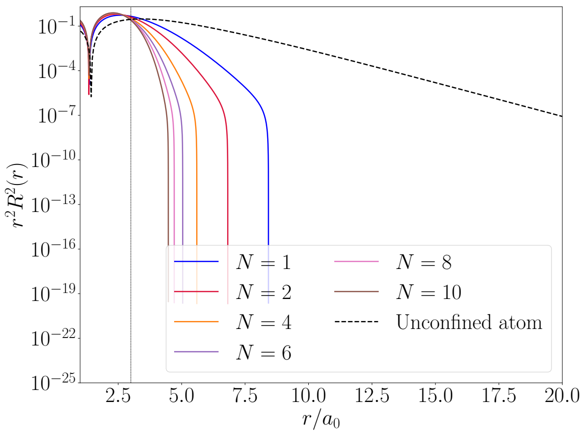


(b)

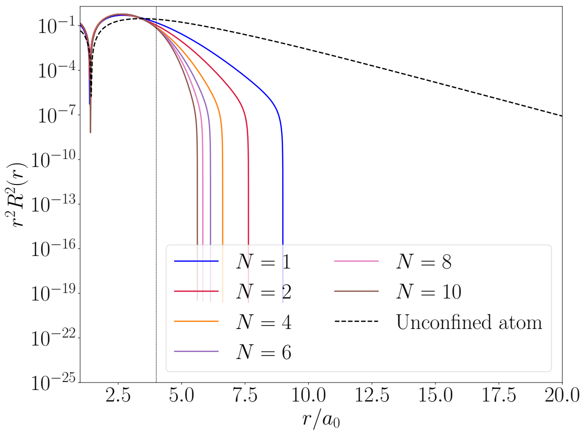


(c)

Figure 20: The radial density of the 4s orbital of Ca in the polynomial potential with a truncated radial grid and $r_0 = 2a_0$ (fig. 20a), $r_0 = 3a_0$ (fig. 20b), and $r_0 = 4a_0$ (fig. 20c).

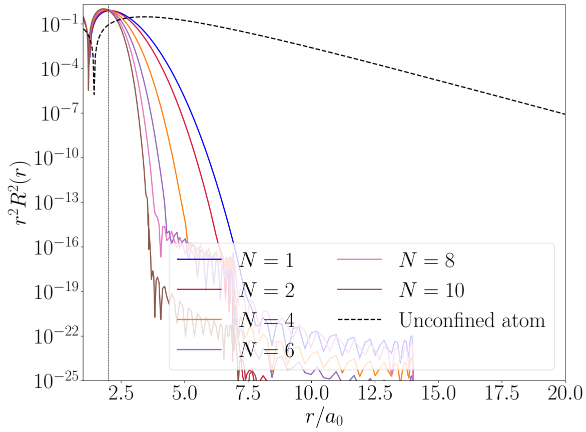


(a)

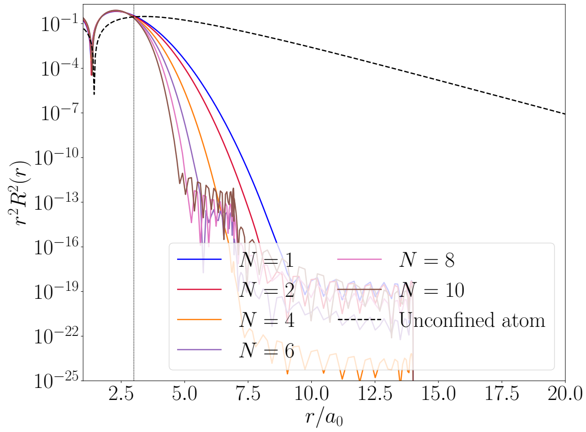


(b)

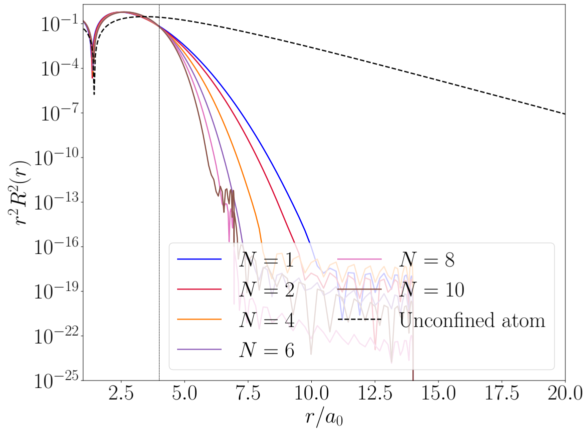


(c)

Figure 21: The radial density of the 4s orbital of Ca in the exponential potential with $r_\infty = 15a_0$ and $r_0 = 2a_0$ (fig. 21a), $r_0 = 3a_0$ (fig. 21b), and $r_0 = 4a_0$ (fig. 21c).

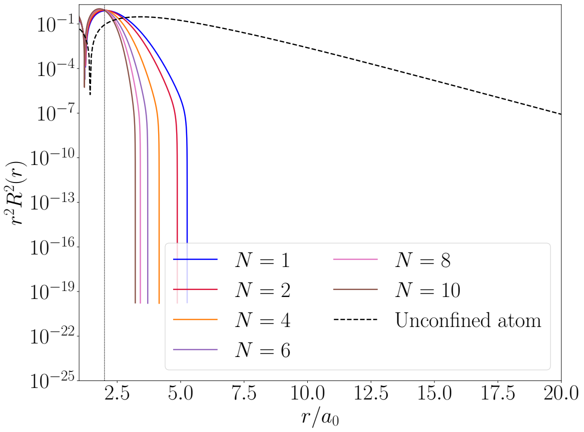


(a)

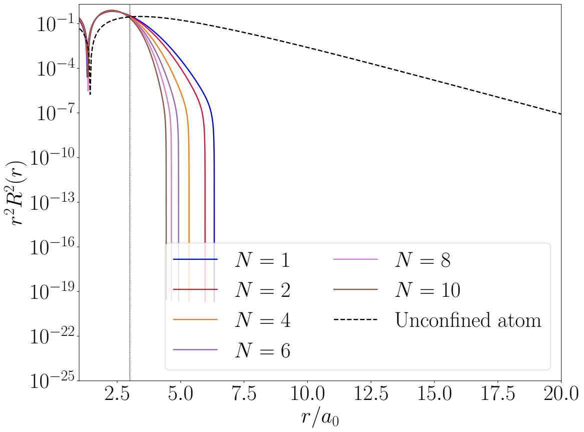


(b)

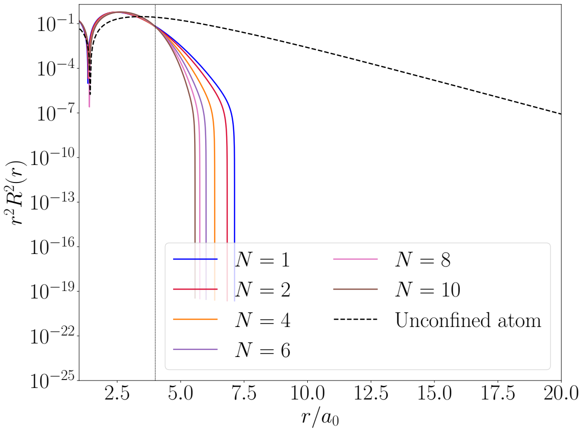


(c)

Figure 22: The radial density of the 4s orbital of Ca in the exponential potential with a truncated radial grid and $r_0 = 2a_0$ (fig. 22a), $r_0 = 3a_0$ (fig. 22b), and $r_0 = 4a_0$ (fig. 22c).

| $N$ | 2 | | 4 | | 6 | | 10 | |
|---|---|---|---|---|---|---|---|---|
| $(r_0, \delta)$ | $r_\infty$ | $\|\|\Delta\|\|$ | $r_\infty$ | $\|\|\Delta\|\|$ | $r_\infty$ | $\|\|\Delta\|\|$ | $r_\infty$ | $\|\|\Delta\|\|$ |
| $(0.1, 4.9)$ | 6.03 | $1.58 \times 10^{-4}$ | 5.55 | $2.26 \times 10^{-5}$ | 5.36 | $5.38 \times 10^{-6}$ | 5.21 | $1.36 \times 10^{-6}$ |
| $(0.2, 4.8)$ | 6.24 | $2.61 \times 10^{-4}$ | 5.73 | $5.37 \times 10^{-5}$ | 5.51 | $1.65 \times 10^{-5}$ | 5.30 | $6.52 \times 10^{-6}$ |
| $(0.3, 4.7)$ | 6.37 | $3.50 \times 10^{-4}$ | 5.84 | $8.78 \times 10^{-5}$ | 5.60 | $2.94 \times 10^{-5}$ | 5.37 | $1.11 \times 10^{-5}$ |
| $(0.5, 4.5)$ | 6.49 | $5.14 \times 10^{-4}$ | 5.98 | $1.63 \times 10^{-4}$ | 5.74 | $6.58 \times 10^{-5}$ | 5.49 | $1.75 \times 10^{-5}$ |
| $(0.7, 4.3)$ | 6.54 | $6.79 \times 10^{-4}$ | 6.06 | $2.47 \times 10^{-4}$ | 5.82 | $1.10 \times 10^{-4}$ | 5.57 | $3.38 \times 10^{-5}$ |
| $(1.0, 4.0)$ | 6.53 | $9.52 \times 10^{-4}$ | 6.11 | $3.92 \times 10^{-4}$ | 5.89 | $1.91 \times 10^{-4}$ | 5.64 | $6.28 \times 10^{-5}$ |
| $(5.0, 0.0)$ | 4.82 | $1.22 \times 10^{-2}$ | 4.90 | $7.40 \times 10^{-3}$ | 5.03 | $4.66 \times 10^{-3}$ | 5.21 | $2.12 \times 10^{-3}$ |

(a) Polynomial

| $N$ | 2 | | 4 | | 6 | | 10 | |
|---|---|---|---|---|---|---|---|---|
| $(r_0, \delta)$ | $r_\infty$ | $\|\|\Delta\|\|$ | $r_\infty$ | $\|\|\Delta\|\|$ | $r_\infty$ | $\|\|\Delta\|\|$ | $r_\infty$ | $\|\|\Delta\|\|$ |
| $(0.1, 4.9)$ | 5.22 | $1.40 \times 10^{-5}$ | 5.16 | $5.09 \times 10^{-6}$ | 5.12 | $2.63 \times 10^{-6}$ | 5.08 | $6.14 \times 10^{-7}$ |
| $(0.2, 4.8)$ | 5.28 | $5.11 \times 10^{-5}$ | 5.23 | $1.56 \times 10^{-5}$ | 5.18 | $8.89 \times 10^{-6}$ | 5.13 | $3.11 \times 10^{-6}$ |
| $(0.3, 4.7)$ | 5.31 | $1.06 \times 10^{-4}$ | 5.27 | $3.73 \times 10^{-5}$ | 5.23 | $1.50 \times 10^{-5}$ | 5.15 | $9.30 \times 10^{-6}$ |
| $(0.5, 4.5)$ | 5.32 | $2.52 \times 10^{-4}$ | 5.32 | $9.95 \times 10^{-5}$ | 5.28 | $4.65 \times 10^{-5}$ | 5.22 | $1.26 \times 10^{-5}$ |
| $(0.7, 4.3)$ | 5.30 | $4.53 \times 10^{-4}$ | 5.33 | $1.86 \times 10^{-4}$ | 5.31 | $8.67 \times 10^{-5}$ | 5.26 | $2.86 \times 10^{-5}$ |
| $(1.0, 4.0)$ | 5.23 | $8.57 \times 10^{-4}$ | 5.33 | $3.73 \times 10^{-4}$ | 5.33 | $1.85 \times 10^{-4}$ | 5.30 | $6.41 \times 10^{-5}$ |
| $(5.0, 0.0)$ | 4.52 | $1.23 \times 10^{-2}$ | 4.77 | $7.37 \times 10^{-3}$ | 4.96 | $4.65 \times 10^{-3}$ | 5.17 | $2.12 \times 10^{-3}$ |

(b) Exponential

Table IV: Values of $r_\infty$ in $a_0$ that minimize the norm between the 4s orbital of the Ca atom in the shifted potentials for various values of $N$, $r_0$ and $\delta$ in $a_0$ and the hard-wall potential.

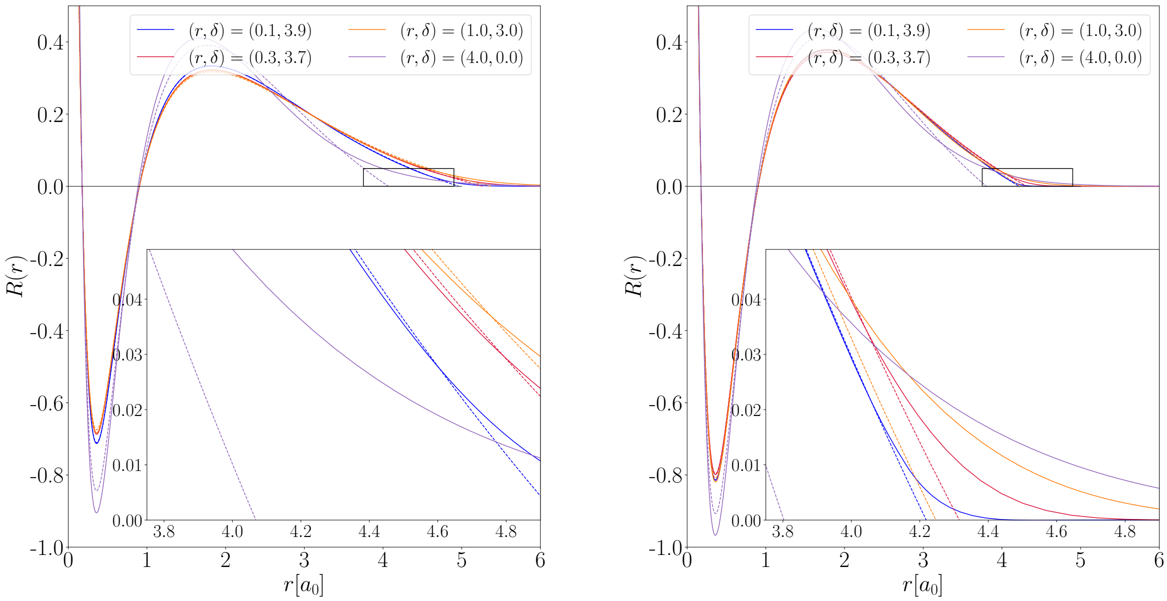


(a) Polynomial.

(b) Exponential.

Figure 23: The radial part of the 3s orbital of the Mg atom confined by the shifted polynomial (fig. 23a) and exponential (fig. 23b) potential with $N = 2$ and varying $r_0$ and $\delta$ (values in parentheses as $(r_0, \delta)$) in solid lines, as well as by the hard-wall potential with various locations of $r_\infty$ in dashed lines.

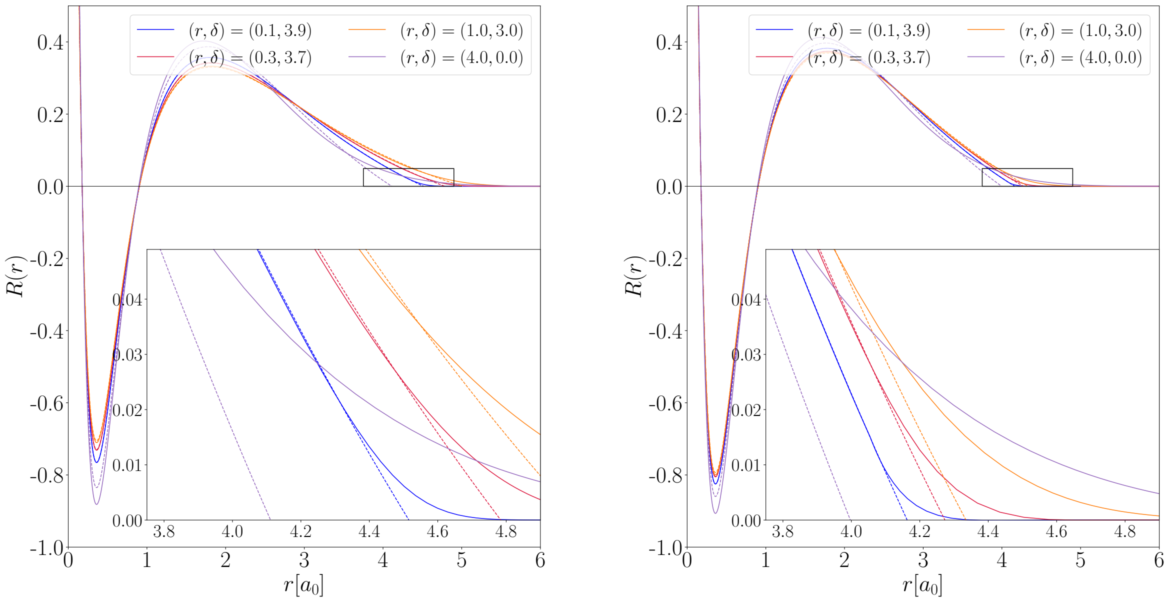


(a) Polynomial.

(b) Exponential.

Figure 24: The radial part of the 3s orbital of the Mg atom confined by the shifted polynomial (fig. 24a) and exponential (fig. 24b) potential with $N = 4$ and varying $r_0$ and $\delta$ (values in parentheses as $(r_0, \delta)$) in solid lines, as well as by the hard-wall potential with various locations of $r_\infty$ in dashed lines.

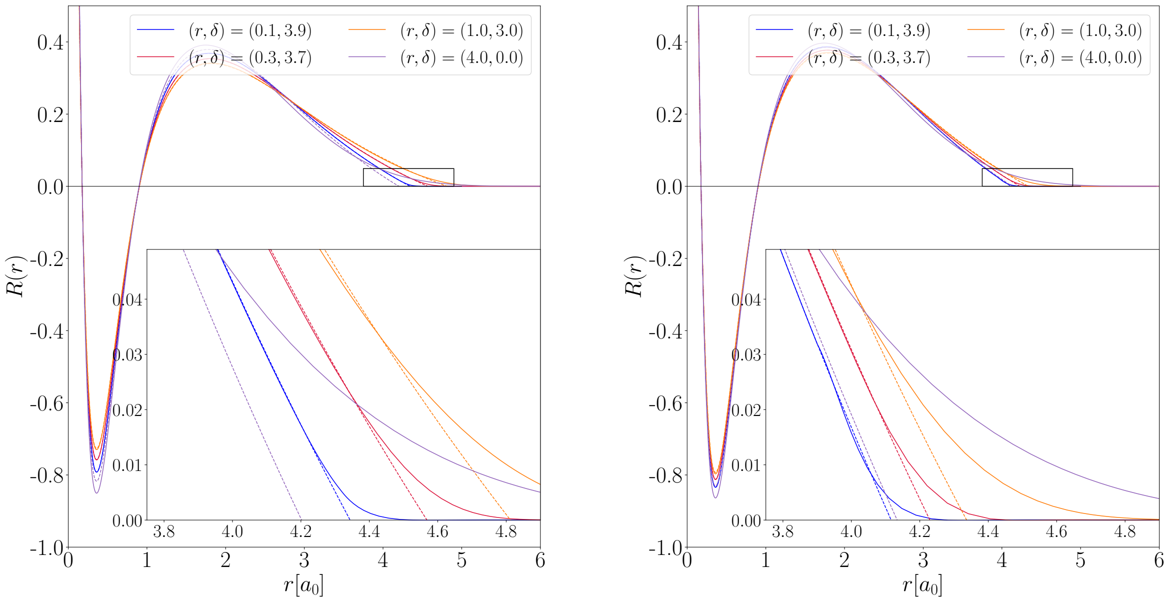


(a) Polynomial.

(b) Exponential.

Figure 25: The radial part of the 3s orbital of the Mg atom confined by the shifted polynomial (fig. 25a) and exponential (fig. 25b) potential with $N = 6$ and varying $r_0$ and $\delta$ (values in parentheses as $(r_0, \delta)$) in solid lines, as well as by the hard-wall potential with various locations of $r_\infty$ in dashed lines.

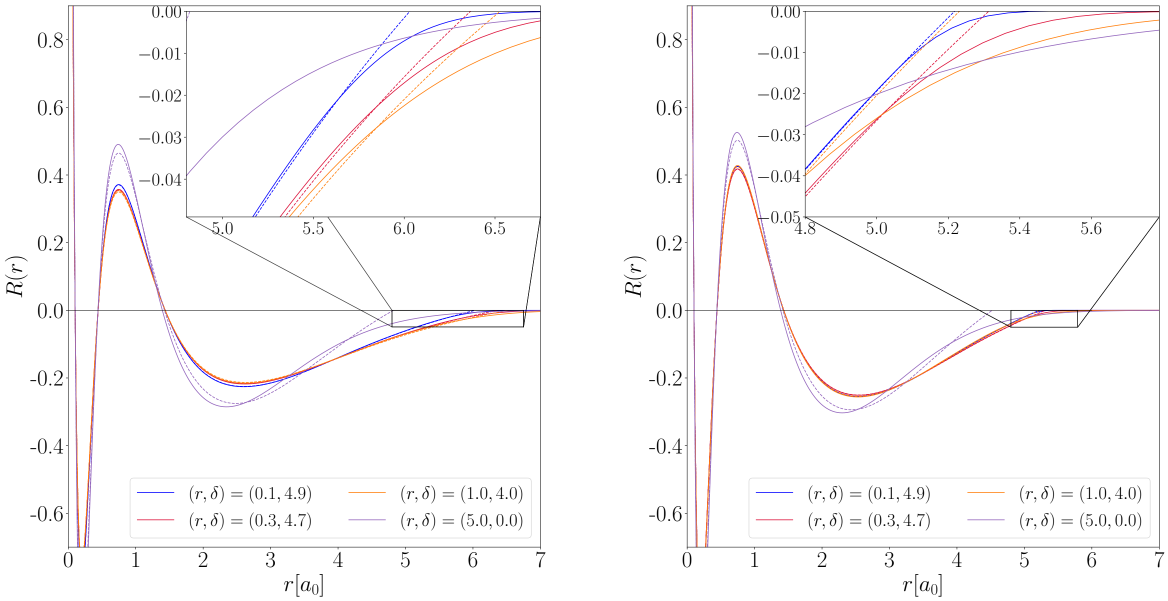


(a) Polynomial.

(b) Exponential.

Figure 26: The radial part of the 4s orbital of the Ca atom confined by the shifted polynomial (fig. 26a) and exponential (fig. 26b) potential with $N = 2$ and varying $r_0$ and $\delta$ (values in parentheses as $(r_0, \delta)$) in solid lines, as well as by the hard-wall potential with various locations of $r_\infty$ in dashed lines.

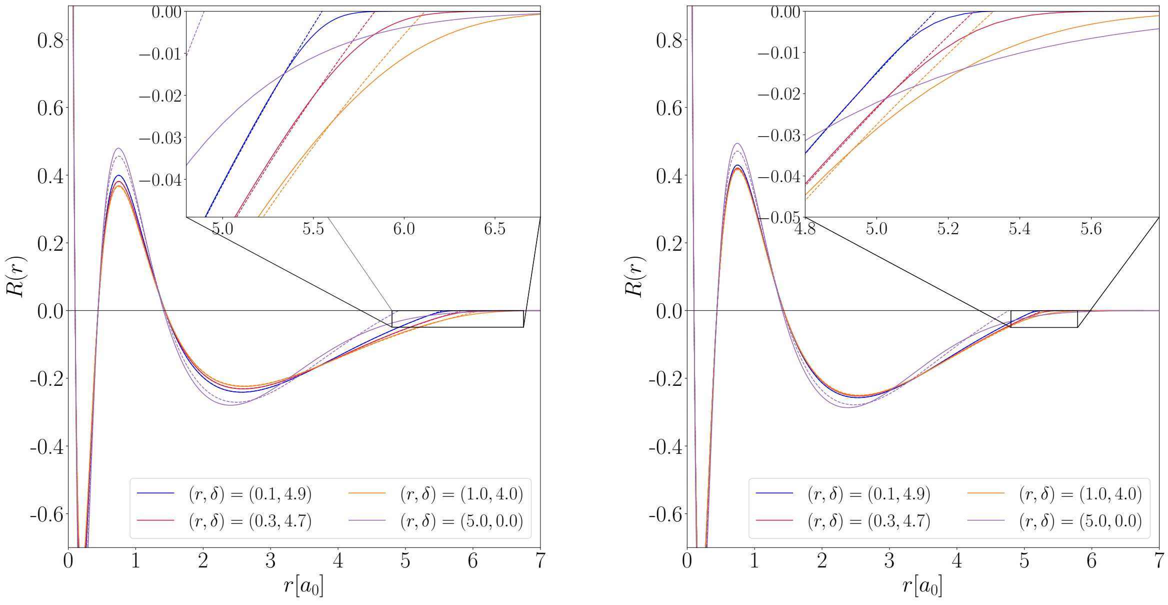


(a) Polynomial.

(b) Exponential.

Figure 27: The radial part of the 4s orbital of the Ca atom confined by the shifted polynomial (fig. 27a) and exponential (fig. 27b) potential with $N = 4$ and varying $r_0$ and $\delta$ (values in parentheses as $(r_0, \delta)$) in solid lines, as well as by the hard-wall potential with various locations of $r_\infty$ in dashed lines.

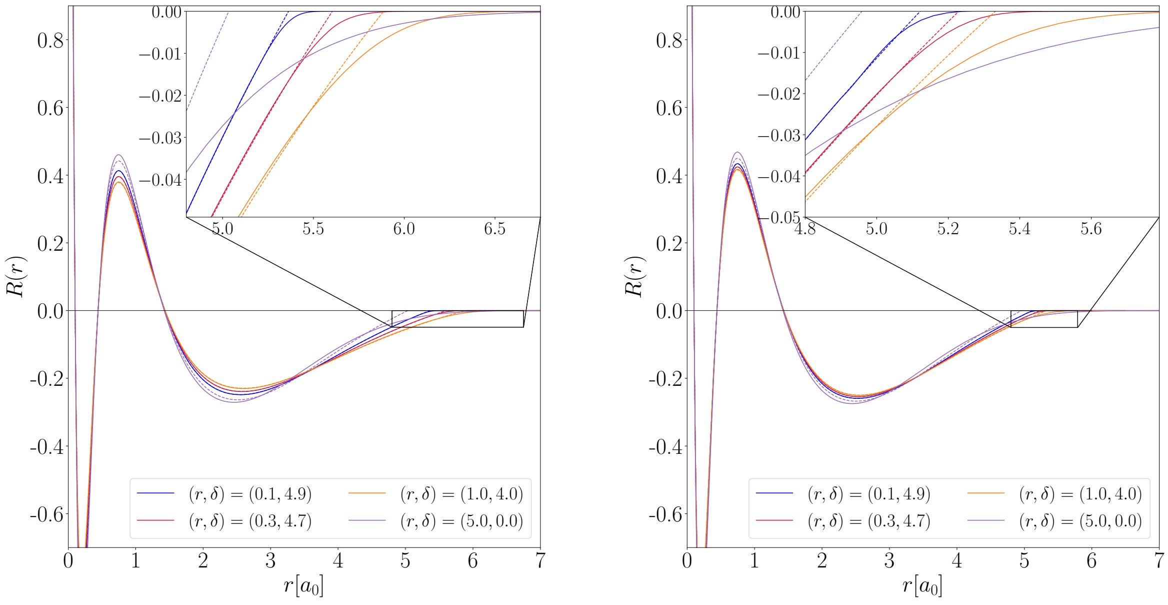


(a) Polynomial.

(b) Exponential.

Figure 28: The radial part of the 4s orbital of the Ca atom confined by the shifted polynomial (fig. 28a) and exponential (fig. 28b) potential with $N = 6$ and varying $r_0$ and $\delta$ (values in parentheses as $(r_0, \delta)$) in solid lines, as well as by the hard-wall potential with various locations of $r_\infty$ in dashed lines.

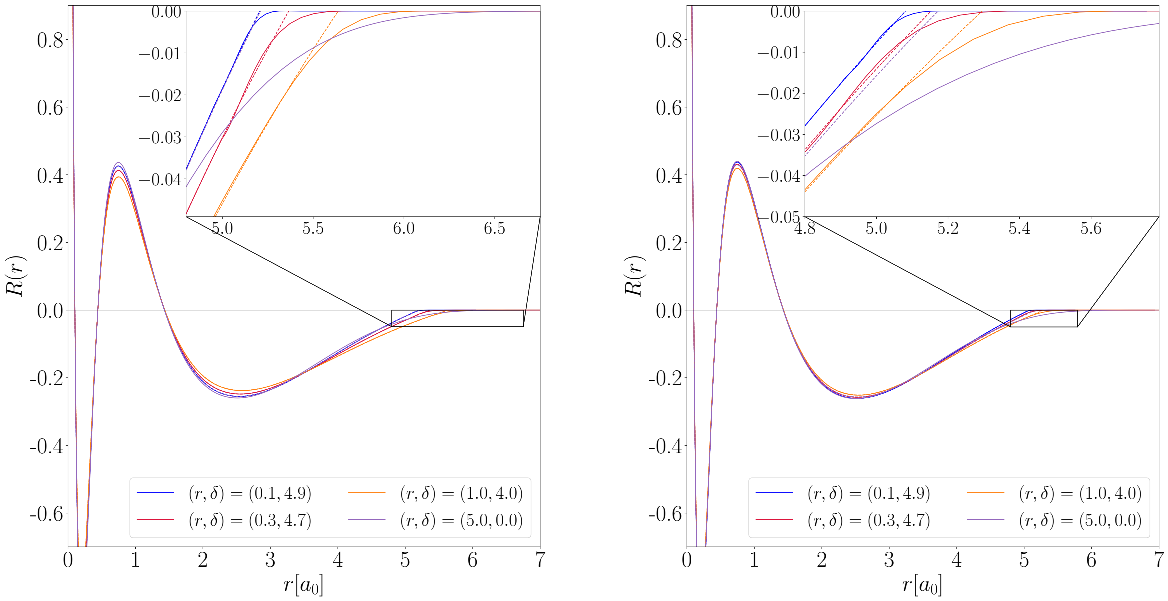


(a) Polynomial.

(b) Exponential.

Figure 29: The radial part of the 4s orbital of the Ca atom confined by the shifted polynomial (fig. 29a) and exponential (fig. 29b) potential with $N = 10$ and varying $r_0$ and $\delta$ (values in parentheses as $(r_0, \delta)$) in solid lines, as well as by the hard-wall potential with various locations of $r_\infty$ in dashed lines.

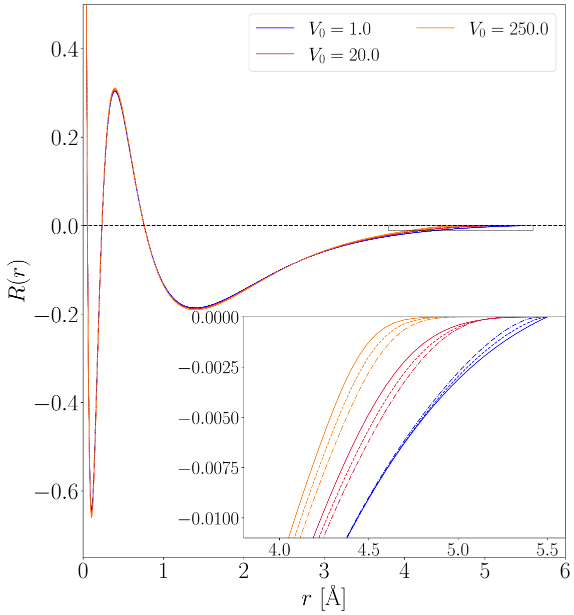


(a) "light" setting

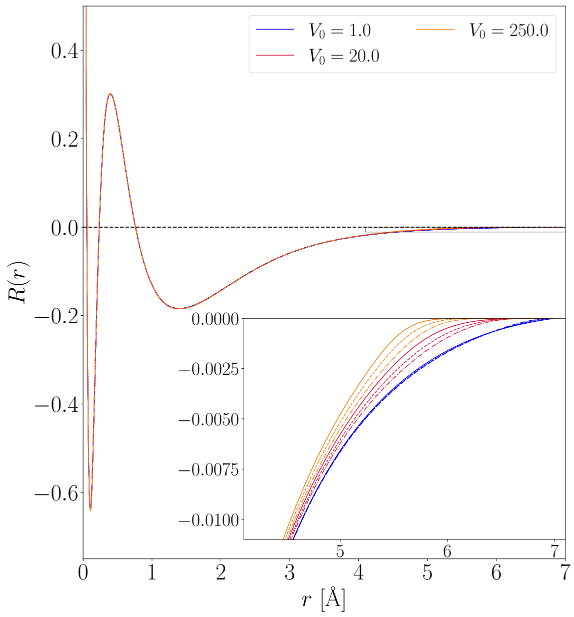


(b) "tight" setting

Figure 30: The radial part of the 4s orbital of Ca confined by the singular potential for $n = 1$ (solid lines), $n = 2$ (dashed lines), and $n = 3$ (dash-dotted lines) and various $V_0$ with the "light" (fig. 30a) and "tight" (fig. 30b) defaults in FHI-AIMS. Note that the unit of $r$ is Å and not $a_0$.

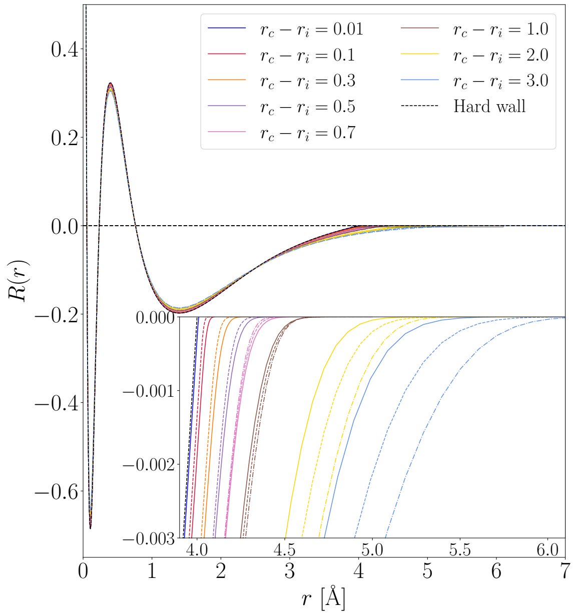


Figure 31: The radial part of the 4s orbital of Ca confined by the singular potential for $n = 1$ (solid lines), $n = 2$ (dashed lines), and $n = 3$ (dash-dotted lines) and various values of $r_c - r_i$ as well as the hard-wall ($r_c - r_i = 0$). Note that the unit of $r$ is Å and not $a_0$.

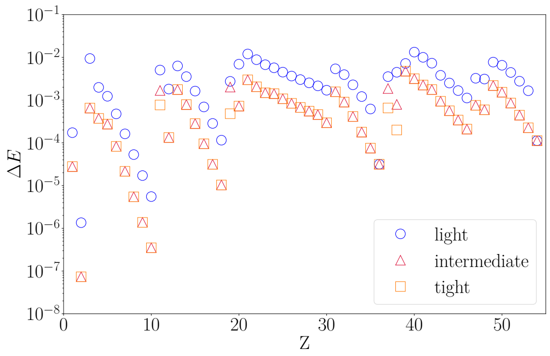


(a) PW92

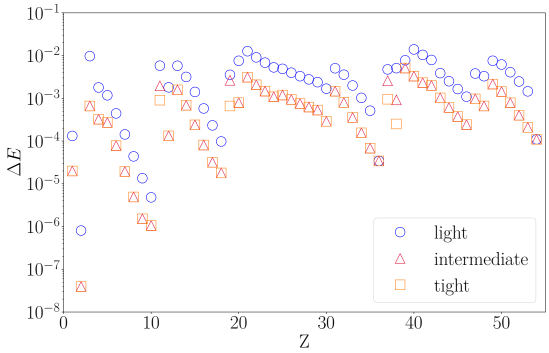


(b) $r^2$SCAN

Figure 32: Truncation errors of the H–Xe atoms with the PW92 (fig. 32a) and $r^2$SCAN (fig. 32b) functionals with the "light", "intermediate", "tight" and "really tight" defaults in FHI-AIMS.
